# Supplementary material for: Physically Accurate Differentiable Inverse Rendering for Radio Frequency Digital Twin
Source: arXiv:2603.18026 source file (2026-03-05)
Supplement: Supplementary file 1 [file appendix.tex]

\section{Differentiable Spatial Specturm}

\label{sec:diff_spect}
In a multiple-input-multiple-output (MIMO) radar system, the angular spectrum can be synthesized through array processing techniques such as beamforming or MUSIC \cite{schmidt1986multiple}. 
Under the far-field assumption, a MIMO array can be viewed equivalently as a single Tx element and a virtual Rx array [cite].

Consider a radar system with a virtual Rx array size of $L$ in a 2D plane.
The received signal can be abstracted as $\mathbf{X}(t)$ with a dimension of $L \times 1$. 
% Steering Vector
The 2D steering vector \( \mathbf{A}(\phi, \theta) \) for each azimuth \( \phi \) and elevation \( \theta \) can be written as:
\[
\mathbf{A}(\phi, \theta) = \begin{bmatrix}
e^{-j \frac{2\pi}{\lambda} \left( x_1 \sin \theta \cos \phi + y_1 \sin \theta \sin \phi \right)} \\
e^{-j \frac{2\pi}{\lambda} \left( x_2 \sin \theta \cos \phi + y_2 \sin \theta \sin \phi \right)} \\
\vdots \\
e^{-j \frac{2\pi}{\lambda} \left( x_{P} \sin \theta \cos \phi + y_{P} \sin \theta \sin \phi \right)}
\end{bmatrix}
\]

\begin{comment}
With a total of $I$ targets, we can rewrite Eq.~\eqref{eq:fmcw_fft} as:
\begin{gather*}
    X[l] = \sum_{i=1}^I a_i e^{j2\pi f_0 \tau_i} g(\tau_i-\tau_l)\\
    \text{where }g(\Delta\tau) = \sum_{n=0}^{N_s-1}e^{j2\pi \frac{Bn\Delta\tau}{N_s}}
\end{gather*}
Here each DFT bin $l$ corresponds to one particular ToF, \ie, $\tau_l = l/B$. 
When a target's range is perfectly aligned with the range bin $l$, $\Delta\tau = 0$ and $g(\Delta\tau) = N_s$ reaches the maximum. 
On the other hand, when a target's range is far from a range bin, $\Delta\tau$ grows large and $|g(\Delta\tau)| \to 0$ following a sinc pattern. 
%Therefore, in an FMCW radar system, information from each range bin is decoupled from each other. 
Notably, $\angle g(\tau_{m,n,i}-\tau_l)$ changes much slower over antenna indices than $2\pi f_0 \tau_{m,n,i}$, and therefore $g(\tau_{m,n,i}-\tau_l)$ can be neglected when performing direction of arrival (DoA) estimation.
\end{comment}

%The impact of $g(\Delta\tau)$ is usually negligible when performing array processing because the phase and gain variations contributed by the $a_{m,n}^{(l)} e^{j2\pi f_0 \tau_{m,n}}$ term is much larger.

\subsubsection{Beamforming-Based Spatial Spectrum}
The beamformed signal at angle $(\phi, \theta)$ can then be computed as:
\begin{equation}
\mathbf{S}(\phi, \theta) = \mathbf{X}^H \mathbf{A}(\phi, \theta)
\end{equation}
The angular spectrum P can be calculated subsequently for all the combinations of $(\theta, \phi)$ as below
\begin{equation}
    \mathbf{P} = \left| \mathbf{S}(\phi, \theta) \right|^2 
\end{equation}

\todo{derivation of Derivatives}

\subsubsection{MUSIC-Based Spatial Spectrum}
MUSIC algorithm is a subspace-based method for DOA estimation and the number of signals $P$ is given as prior knowledge. 

The first step is estimating the covariance matrix of the signals across all the antenna elements. 
% Covariance Matrix Computation
Suppose $T$ snapshots are taken, and the covariance matrix \( R \) can be computed as:

\begin{equation}
\hat{\mathbf{R}} = \frac{1}{T} \sum_{t=1}^{T} \mathbf{X}(t) \mathbf{X}^H(t)
\end{equation}

% Eigenvalue Decomposition
Perform eigenvalue decomposition on the estimated covariance matrix \( \hat{\mathbf{R}} \):

\begin{equation}
    \hat{\mathbf{R}} \mathbf{U} = \mathbf{U} \mathbf{D}
\end{equation}

where \( \mathbf{D} \) is a diagonal matrix of eigenvalues, and \( \mathbf{U} \) is the matrix of corresponding eigenvectors.

Sort the eigenvalues \( \lambda_i \) in descending order, and arrange the eigenvectors correspondingly:
\[
\lambda_1 \geq \lambda_2 \geq \cdots \geq \lambda_{L}
\]
% Signal and Noise Subspaces
The signal subspace \( \mathbf{U}_s \) and noise subspace \( \mathbf{U}_n \) are defined as:
\[
\mathbf{U}_s = \left[ \mathbf{U}(:,1), \mathbf{U}(:,2), \ldots, \mathbf{U}(:,P) \right]
\]
\[
\mathbf{U}_n = \left[ \mathbf{U}(:,P+1), \mathbf{U}(:,P+2), \ldots, \mathbf{U}(:,L) \right]
\]

% MUSIC Pseudospectrum
The MUSIC pseudo spectrum \( S(\phi, \theta) \) is calculated by:

\begin{equation}
\small
   S(\phi_i, \theta_j) = \frac{1}{\mathbf{A}(\phi_i, \theta_j)^H \mathbf{U}_n \mathbf{U}_n^H \mathbf{A}(\phi_i, \theta_j)} 
\end{equation}

This equation is computed for all combinations of azimuth and elevation angles \( (\phi_i, \theta_j) \).
\todo{derivation of Derivatives}
